# Supplementary material for: Exceptional magic angles in non-Hermitian twisted bilayer graphene
Source: arXiv:2408.08804 source file (2025-06-04)
Supplement: Supplementary file 1 [file SM.pdf]

# Supplementary Information: “Exceptional magic angles in non-Hermitian twisted bilayer graphene”

Juan Pablo Esparza<sup>1,2</sup> and Vladimir Juričić<sup>1</sup>

<sup>1</sup>*Departamento de Física, Universidad Técnica Federico Santa María, Casilla 110, Valparaíso, Chile*

<sup>2</sup>*Instituto de Física, Pontificia Universidad Católica de Valparaíso,  
Avenida Universidad 331, Curauma, Valparaíso, Chile*

In this Supplementary Information, we present the following: (S1) Explicit derivation of the density of states for the non-Hermitian Dirac Hamiltonian in Eq. (1) in the main text; (S2) Details of the biorthogonal basis of the non-Hermitian Dirac Hamiltonian for the monolayer graphene; (S3) Derivation of the continuum model for non-Hermitian twisted bilayer graphene; (S4) Calculation of the Berry phase of the non-Hermitian Dirac Hamiltonian; (S5) Additional plots of the band structure and Fermi velocity for the non-Hermitian twisted bilayer graphene; (S6) Analysis of alternative models of non-Hermitian twisted bilayer graphene; (S7) Details of the experimental proposal.

## S1. DENSITY OF STATES OF THE NH DIRAC FERMIONS

We start by the definition of the density of states for  $N_f$  copies of two-component Dirac fermions with generic dispersion relation  $\epsilon_{s,\mathbf{k}}$ ,

$$\rho(\epsilon) = N_f \sum_s \int \frac{d^d \mathbf{k}}{(2\pi)^d} \delta[\epsilon - \text{Re}(\epsilon_{s,\mathbf{k}})].$$

Notice that the density of states is non-zero only when the dispersion  $\epsilon_{s,\mathbf{k}}$  possesses the real part. Replacing the energy-momentum relation of our model for non-Hermitian Dirac Hamiltonian in Eq. (1) of the main text, holding for the energies  $|\epsilon| \leq \Lambda$ , with  $\Lambda$  as the cutoff scale (typically, given by the bandwidth of the underlying lattice model),  $\epsilon_{s,\mathbf{k}} = sv_H \sqrt{1 - \beta^2} |\mathbf{k}| \equiv skv_F$ , with  $\beta = v_{\text{NH}}/v_H$ , and taking  $d = 2$ , with  $s = +$  ( $s = -$ ) as the band index corresponding to the conduction (valence) band, then for  $\epsilon > 0$ , leads to

$$\begin{aligned} \rho(\epsilon) &= N_f \sum_{s=\pm} \int_0^{2\pi} \frac{d\theta}{(2\pi)^2} \int_0^{\Lambda/v_F} dk k \delta[\epsilon - sk \text{Re}(v_F)] \\ &= \frac{N_f}{2\pi} \int_0^{\Lambda/v_F} dk k \delta[\epsilon - \text{Re}(v_F) k] \\ &= \frac{N_f}{2\pi v_F^2} \Theta(1 - |\beta|) \int_0^\Lambda dx x \delta(\epsilon - sx) \\ &= N_f \frac{\epsilon}{2\pi v_F^2} \Theta(1 - |\beta|). \end{aligned}$$

Here, in the first step we just evaluate the integral over  $\theta$ , and we then make the substitution  $x = v_F k$ , with a Heaviside step-function  $\Theta(1 - |\beta|)$  ensuring that the real part of the dispersion, inherited from the reality condition for  $v_F$ , is non-zero. Similarly, for  $\epsilon < 0$ , we find

$$\rho(\epsilon) = -N_f \frac{\epsilon}{2\pi v_F^2} \Theta(1 - |\beta|),$$

and therefore we can compactly write

$$\rho(\epsilon) = N_f \frac{|\epsilon|}{2\pi v_F^2} \Theta(1 - |\beta|).$$

On the other hand, when the dispersion is purely imaginary, thus  $|\beta| > 1$ , the density of states is

$$\begin{aligned} \rho(\epsilon) &= 2N_f \Theta(|\beta| - 1) \delta(\epsilon) \int_0^{2\pi} \frac{d\theta}{(2\pi)^2} \int_0^{\Lambda/v_F} dk k \\ &= N_f \frac{\Lambda^2}{2\pi v_F^2} \Theta(|\beta| - 1) \delta(\epsilon). \end{aligned}$$

Taking into account both cases, we can therefore write the density of states as

$$\rho(\epsilon) = \frac{N_f}{2\pi v_F^2} \{ |\epsilon| \Theta(1 - |\beta|) + \Lambda^2 \delta(\epsilon) \Theta(|\beta| - 1) \}, \quad (\text{S1})$$

which is the result shown in the paragraph after Eq. (2) of the main text. Notice that a sharp peak at  $\epsilon = 0$  emerges at the exceptional points  $|\beta| = 1$ , which signals the band flattening taking place.

As a final comment, we notice that the total number of states per unit volume,  $\mathfrak{n}$ , does not change as the system crosses any of the two exceptional points at  $|\beta| = 1$ :

$$\mathfrak{n} = \int_{-\Lambda}^{\Lambda} d\epsilon \rho(\epsilon) \Big|_{|\beta| < 1} = \int_{-\Lambda}^{\Lambda} d\epsilon \rho(\epsilon) \Big|_{|\beta| > 1} = N_f \frac{\Lambda^2}{2\pi v_F^2}.$$

## S2. BIORTHOGONAL BASIS AND EXCEPTIONAL POINTS

To obtain the right- and left-eigenstates of  $h_{\mathbf{k}}$  that constitutes the biorthogonal basis for the system [1], we must solve the eigenvalue problem

$$\left( h_{\mathbf{k}} - \epsilon_{\mathbf{k}}^{(s)} \right) \psi_R^{(s)}(\mathbf{k}) = 0, \quad \left( h_{\mathbf{k}}^\dagger - \epsilon_{\mathbf{k}}^{(s)} \right) \psi_L^{(s)}(\mathbf{k}) = 0 \quad (\text{S2})$$

for  $s = \pm$  and  $\epsilon_{\mathbf{k}}^{(s)} = sv_F |\mathbf{k}|$ , with  $v_F = \sqrt{v_H^2 - v_{\text{NH}}^2}$ . To visualize the difference between both equations, it will be convenient to write  $h_{\mathbf{k}}$  explicitly in a closed matrix form as

$$h_{\mathbf{k}}(v_+, v_-) = \begin{pmatrix} 0 & v_+ |\mathbf{k}| e^{-i\theta_{\mathbf{k}}} \\ v_- |\mathbf{k}| e^{i\theta_{\mathbf{k}}} & 0 \end{pmatrix}, \quad (\text{S3})$$

where we define  $v_{\pm} = v_H \pm v_{NH}$ . It becomes evident now that the only difference between  $h_{\mathbf{k}}$  and its complex conjugate is just the replacement  $v_+ \leftrightarrow v_-$ , and thus is enough to solve one of the eigenproblems in Eq. (S2). A straightforward algebra then leads to the normalized solutions

$$\begin{aligned}\psi_R^{(s)}(\mathbf{k}) &= \frac{1}{\sqrt{2v_F}} \begin{pmatrix} \sqrt{v_+} \\ s\sqrt{v_-}e^{i\theta_{\mathbf{k}}} \end{pmatrix}, \\ \psi_L^{(s)}(\mathbf{k}) &= \frac{1}{\sqrt{2v_F}} \begin{pmatrix} \sqrt{v_-} \\ s\sqrt{v_+}e^{i\theta_{\mathbf{k}}} \end{pmatrix}.\end{aligned}\quad (\text{S4})$$

Notice that the condition  $v_F = 0$  is ill-defined for both eigenstates, since it appears as a normalization factor. Moreover, if we rewrite  $v_F = \sqrt{v_+v_-}$  it becomes transparent that, in order to get  $v_F = 0$ , necessarily either  $v_+ = 0$  or  $v_- = 0$  (since they cannot be zero simultaneously for  $v_{NH} \neq 0$ ). In both cases, the Hamiltonian  $h_{\mathbf{k}}$  becomes defective (see Eq. (S3)), and the linearly independent eigenstates coalesce to the same vector. Consequently, we identify the condition  $v_F = 0$  as an *exceptional point*. This can be understood as a consequence of the non-monotonic dependence of the spectrum (through  $v_F$ ) on the parameters  $v_{\pm}$  (or  $v_H$  and  $v_{NH}$ ), a typical characteristic of non-Hermitian systems [2, 3].

To explicitly demonstrate this, we take  $v_+ = 0$  in Eq. (S3), which then becomes

$$h_{\mathbf{k}}(0, v_-) = v_- |\mathbf{k}| e^{i\theta_{\mathbf{k}}} \begin{pmatrix} 0 & 0 \\ 1 & 0 \end{pmatrix}.$$

This matrix obviously has a doubly degenerate eigenvalue equal to zero but only one corresponding eigenvector equal to  $(0, 1)^T$ , showing its defectiveness. The same analysis shows that  $h_{\mathbf{k}}(v_+, 0)$  is also defective, therefore implying that the condition  $v_F = 0$  corresponds to an exceptional point of the non-Hermitian Dirac Hamiltonian in Eq. (S3).

### S3. DERIVATION OF THE CONTINUUM MODEL FOR NON-HERMITIAN TWISTED BILAYER GRAPHENE

Starting from the low-energy Hamiltonian in Eq. (3) of the main text, we follow the approach of Bistritzer-MacDonald [4], which consists in taking the momentum-dependent part of the Hamiltonian as a perturbation of the momentum-independent part encoding the inter-layer hybridization. Specifically, we separate  $\mathcal{H}_{\mathbf{k}} = \mathcal{H}^{(0)} + \mathcal{H}^{(1)}$ , with

$$\mathcal{H}^{(0)} = \begin{pmatrix} h_0 & T_1 & T_2 & T_3 \\ T_1 & h_{-\mathbf{q}_1} & 0 & 0 \\ T_2 & 0 & h_{-\mathbf{q}_2} & 0 \\ T_3 & 0 & 0 & h_{-\mathbf{q}_3} \end{pmatrix} \quad (\text{S5})$$

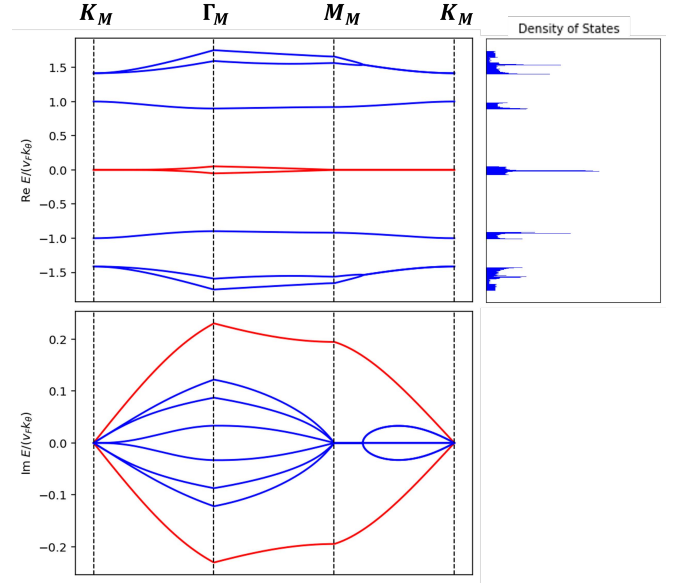

Figure S1. Real (top) and imaginary (bottom) parts of the energy bands for the 8-band model for  $w_0 = 0$  at the Hermitian magic angle,  $\alpha_1 = 1/\sqrt{3}$ . We use the values of the in-plane velocities  $v_F = 1$  and  $v_{NH} = 0.5$ . Notice that the imaginary part of the flattened bands in real energy is significantly larger than its counterpart at the exceptional magic angles, and is clearly not flat in the vicinity of the  $K_M$  point.

and

$$\mathcal{H}^{(1)} = \mathbf{1}_4 \otimes (v_H + v_{NH}\sigma_3)\boldsymbol{\sigma} \cdot \mathbf{k}. \quad (\text{S6})$$

Then, to concentrate on the lowest energy bands, we look for zero-energy eigenstates of  $\mathcal{H}^{(0)}$ . Since the operator is non-Hermitian, we also need to consider both its right and left eigenstates, defined by

$$\Psi_L^\dagger \mathcal{H}^{(0)} = 0, \text{ and } \mathcal{H}^{(0)} \Psi_R = 0.$$

Focusing on the right eigenstate, which we may write as  $\Psi_R = (\psi_0, \psi_1, \psi_2, \psi_3)^T$ , the direct operation of the Hamiltonian leads to the system of equations

$$\begin{aligned}h_0\psi_0 + \sum_j T_j\psi_j &= 0, \\ T_j\psi_0 + h_j\psi_j &= 0,\end{aligned}$$

where we define  $h_j = h_{-\mathbf{q}_j}$  for notational simplicity, and  $j = 1, 2, 3$ . From the second equation, we may obtain an expression for  $\psi_j$  in terms of  $\psi_0$  and replace it in the first one. Such substitution leads to the eigenvalue problem

$$(h_0 - \sum_j T_j h_j^{-1} T_j) \psi_0 = 0.$$

In the hermitian case,  $\sum_j T_j h_j^{-1} T_j = 0$  and  $\psi_0$  is precisely the zero-energy eigenstate of the single-layer operator  $h_0$  [4]. In our case, an explicit calculation gives

$\sum_j T_j h_j^{-1} T_j = i \frac{6w_0 w_1 k_\theta}{v_F^2 k_\theta^2} v_{\text{NH}}$ , so  $\psi_0$  is an eigenstate with zero real part of energy of the non-Hermitian single-layer operator, but with a displacement in the imaginary part proportional to the product of dimensionless parameters  $\alpha_0$  and  $\alpha_1$ , and the non-Hermitian velocity  $v_{\text{NH}}$ . Thus, the complete solution for the right eigenstate can be written explicitly as

$$\Psi_R = \begin{pmatrix} \psi_0 \\ -h_1^{-1} T_1 \psi_0 \\ -h_2^{-1} T_2 \psi_0 \\ -h_3^{-1} T_3 \psi_0 \end{pmatrix}, \quad (\text{S7})$$

and following the exact same argument for the the left eigenstate we find

$$\Psi_L^\dagger = (\psi_0^\dagger \quad -\psi_0^\dagger T_1 h_1^{-1} \quad -\psi_0^\dagger T_2 h_2^{-1} \quad -\psi_0^\dagger T_3 h_3^{-1}), \quad (\text{S8})$$

which are the eigenstates displayed in Eq. (8) of the main text.

Finally, with this biorthogonal basis, we apply the standard perturbation theory to obtain the form of the momentum-dependent part of the Hamiltonian,  $\mathcal{H}^{(1)}$ , in the previously obtained basis,

$$\langle i | \mathcal{H}^{(1)} | j \rangle = \frac{\Psi_L^{(i)\dagger} \mathcal{H}^{(1)} \Psi_R^{(j)}}{\Psi_L^{(i)\dagger} \Psi_R^{(j)}}. \quad (\text{S9})$$

An explicit calculation of the denominator then yields

$$\begin{aligned} \Psi_L^\dagger \Psi_R &= \psi_{0,L}^\dagger \psi_{0,R} + \psi_{0,L}^\dagger \sum_j T_j (h_j^{-1})^2 T_j \psi_{0,R} \\ &= \psi_{0,L}^\dagger \psi_{0,R} + \psi_{0,L}^\dagger \left( (v_F^2 k_\theta^2)^{-1} \sum_j T_j^2 \right) \psi_{0,R} \\ &= 1 + 3 \frac{(w_0^2 + w_1^2)}{v_F^2 k_\theta^2} \equiv 1 + 3(\alpha_0^2 + \alpha_1^2), \end{aligned} \quad (\text{S10})$$

where we use that the biorthogonal basis vectors are normalized,  $\psi_{0,L}^\dagger \psi_{0,R} = 1$ . Equivalently, the numerator can be directly computed as

$$\Psi_L^\dagger \mathcal{H}^{(1)} \Psi_R = \psi_{0,L}^\dagger h_{\mathbf{k}} \psi_{0,R} + \psi_{0,L}^\dagger \sum_j T_j h_j^{-1} h_{\mathbf{k}} h_j^{-1} T_j \psi_{0,R}. \quad (\text{S11})$$

Focusing on the second term, after some straightforward algebra, we obtain

$$\sum_j T_j h_j^{-1} h_{\mathbf{k}} h_j^{-1} T_j = -3\alpha_1^2 h_{\mathbf{k}}^\dagger,$$

which ultimately yields for the numerator of the effective Hamiltonian in Eq. (S9),

$$\begin{aligned} \Psi_L^\dagger \mathcal{H}^{(1)} \Psi_R &= \psi_{0,L}^\dagger \left( h_{\mathbf{k}} - 3\alpha_1^2 h_{\mathbf{k}}^\dagger \right) \psi_{0,R} \\ &= \psi_{0,L}^\dagger [v_H(1 - 3\alpha_1^2) + v_{\text{NH}}(1 + 3\alpha_1^2)\sigma_3] \boldsymbol{\sigma} \cdot \mathbf{k} \psi_{0,R}. \end{aligned} \quad (\text{S12})$$

Finally, replacing Eqs. (S12) and (S10) into Eq. (S9) yields the effective Hamiltonian in Eq. (11) of the main text, with the corresponding renormalized velocities as given in Eq. (12).

#### S4. QUANTIZATION OF THE BERRY PHASE

The generalization of the Berry connection to non-Hermitian systems in the biorthogonal basis reads [5],

$$\mathbf{A}(\mathbf{k}) = -i\psi_L^\dagger(\mathbf{k}) \nabla_{\mathbf{k}} \psi_R(\mathbf{k}). \quad (\text{S13})$$

For our model, a direct substitution of Eq. (S4) yields the standard representation of the two-dimensional gauge potential for a vortex located at the origin

$$\mathbf{A}(\mathbf{k}) = \frac{1}{2|\mathbf{k}|} \hat{\mathbf{e}}_{\theta_{\mathbf{k}}}, \quad (\text{S14})$$

which exhibits non-trivial vorticity and thus implies a quantization of the Berry phase over a closed curve  $C$  in the BZ as

$$\gamma(C) = \oint_C \mathbf{A}(\mathbf{k}) \cdot d\mathbf{k} = \pi. \quad (\text{S15})$$

Remarkably, these quantities possess the exact same value in the Hermitian Dirac Hamiltonian, without being modified by the non-Hermitian piece in the Hamiltonian operator. Finally, as also outlined in the main text, non-spatial unitary and antiunitary particle-hole symmetries (PHS) protect the form of the NH Dirac Hamiltonian:

1. Unitary PHS,  $\mathcal{S} h_{\mathbf{k}} \mathcal{S}^{-1} = -h_{\mathbf{k}}$ , with  $\mathcal{S} = \sigma_3$ .
2. Anti-unitary PHS,  $\mathcal{C}_- h_{\mathbf{k}}^\dagger \mathcal{C}_-^{-1} = -h_{\mathbf{k}}$ , with  $\mathcal{C}_- = \sigma_1 \mathcal{K}$ ;
3. Conjugate time-reversal symmetry  $(\text{TRS}^\dagger)$ ,  $\mathcal{C}_+ h_{\mathbf{k}}^\dagger \mathcal{C}_+^{-1} = h_{\mathbf{k}}$ , with  $\mathcal{C}_+ = \sigma_2 \mathcal{K}$ , where  $\mathcal{K}$  is the complex conjugation;
4. The composite  $C_2 \mathcal{T}$  symmetry, with  $C_2$  ( $\mathcal{T}$ ) as the two-fold rotation (time-reversal), represented by  $\sigma_1$  ( $\mathcal{K}$ ), maps the NH Dirac Hamiltonian  $H(\mathbf{k})$  into  $H^\dagger(\mathbf{k})$ ,  $C_2 \mathcal{T} H(\mathbf{k}) C_2 \mathcal{T} = H^\dagger(\mathbf{k})$ .

#### S5. ADDITIONAL FIGURES

For completeness, here we show additional plots that further corroborate our results. First, we include the band structure plots in the 8-band model (Eq. (3) in the main text) for the Hermitian magic angle (HMA) in Fig. S1 and the second exceptional magic angle (EMA) in Fig. S2. The analogous band structure plots for the

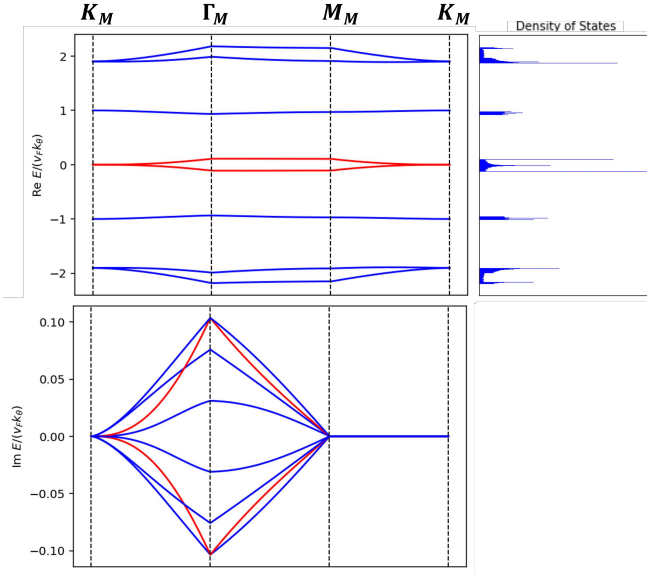

Figure S2. Numerical results for the bands at the second EMA, following the highly symmetrical path on the mBZ. Both real (top panel) and imaginary (bottom panel) components of the quasi-zero modes become flat near the  $K_M$ -point, giving rise to a sharp peak in the DOS. There is, however, a strong degeneracy of the imaginary part along the path  $M_M \rightarrow K_M$ , where all the bands become purely real.

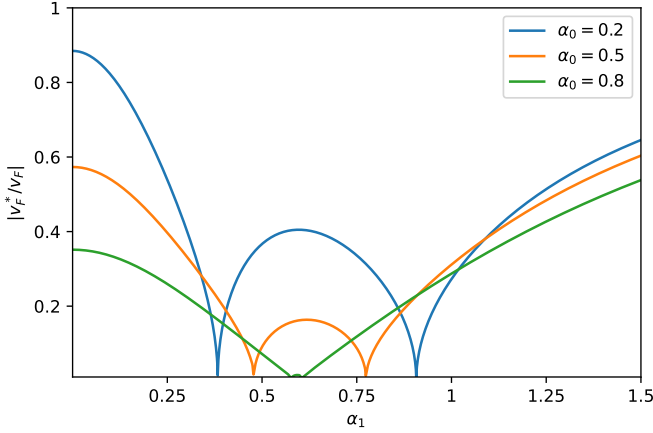

Figure S3. Absolute value of the effective Fermi velocity in the 8-band continuum model in the non-chiral limit,  $\alpha_0 \neq 0$ . Remarkably, increasing  $\alpha_0$  leads to a reduction of the distance between the two exceptional magic angles (EMAs) as  $v_{\text{NH}}^*$  decreases, in agreement with the effective NH TBG Dirac model. The value of the Hermitian magic angle is not modified, which is also consistent with our findings.

first EMA are shown in Fig. 3 of the main text. Notably, at the second EMA a strong degeneracy of the imaginary part along the path  $M_M \rightarrow K_M$  can be observed. Furthermore, we also notice a small gap opened between the closest-to-zero-energy bands but only along the path  $\Gamma_M \rightarrow M_M$ , that is an order of magnitude smaller than the gap to the next bands in the mBZ. This feature there-

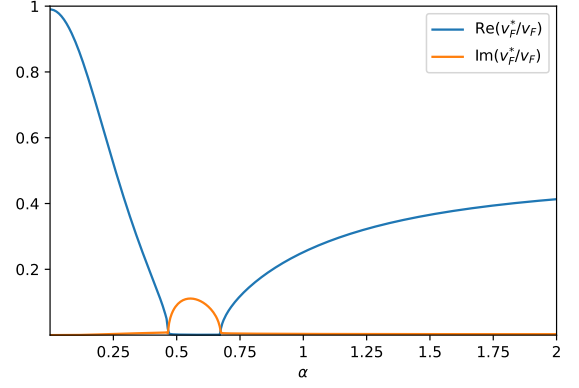

Figure S4. Real and imaginary parts of the renormalized Fermi velocity for the isotropic limit,  $\alpha_0 = \alpha_1 \equiv \alpha$ . The phenomenology is practically identical to the chiral model, being either purely real or purely imaginary, with the HMA as the point for which  $\text{Im}(v_F^*/v_F)$  reaches its maximum value.

fore only weakly perturbs the flatness of the closest-to-zero-energy bands.

The bands close to the HMA, displayed in Fig. S1, show the flattening in the real part of the energy, with the imaginary part exhibiting a bandwidth which is an order of magnitude larger than close to the first EMA (Fig. 3 in the main text), therefore implying much shorter lifetime of the electronic states close to the HMA than to the EMAs. This feature is qualitatively consistent with the predicted increase of the imaginary energy from the NH Dirac model [Eqs. (11) and (12) of the main text]. These features remain when the intra-sublattice interlayer hopping,  $\alpha_0 \neq 0$ , is included, as explicitly shown in Figs. S3 to S5. However, such a PHS breaking term shrinks the region between the two EMAs, with a critical value of  $\alpha_0 \simeq 0.8$  at which the EMAs merge to the HMA, as explicitly shown in Fig. S3. On the other hand, the value of the HMA is robust to the PHS breaking term. This conclusion is further corroborated by the analysis of the 8-band model in the isotropic limit,  $w_0 = w_1$ , exhibiting a similar phenomenology as the chiral one, as shown in Fig. S4. Most importantly, the isotropic model exhibits a shift in the imaginary energy at which the bands touch at the  $K_M$  point, consistent with the continuum theory, Eq. (7) of the main text. Finally, in Fig. S5 we include band plots for the HMA in the non-chiral model,  $\alpha_0 \neq 0$ , to emphasize the effect of such parameter on the imaginary part of the spectrum, which reaches its maximum value precisely at the HMA. The main effect of taking  $\alpha_0 \neq 0$  is a mere shift in the imaginary part of the zero-energy bands, which is consistent with the eigenvalue problem obtained for the quasi-zero modes of the full NH TBG model (see Eq. (7) of the main text), which exhibits a shift in the imaginary part of energy proportional to  $\alpha_0$ .

## S6. ALTERNATIVE MODELS OF NON-HERMITIAN TWISTED BILAYER GRAPHENE

To support the robustness of our results, here we analyze two alternative approaches to obtain non-Hermitian versions of twisted bilayer graphene, by including two different types of on-site dissipation.

First, consider two layers of graphene with balanced gain-loss, so one layer is submitted to gain and the other to loss, with the same parameter  $\gamma$ , and the effective single-layer Hamiltonian in the vicinity of the Dirac points given by

$$h_{\mathbf{k}}^{(s)} = v\boldsymbol{\sigma} \cdot \mathbf{k} + is\gamma, \quad (\text{S16})$$

where  $s = \pm$  is the layer index so that top layer with  $s = +$  (bottom layer with  $s = -$ ) features gain (loss). The spectrum is given by  $\epsilon_{\mathbf{k}}^{(s)} = v|\mathbf{k}| + is\gamma$ , so the parameter  $\gamma$  yields a non-unitary evolution of states at each layer. Notice that the reality of the spectrum depends only on the condition  $\gamma \neq 0$ , and consequently one may expect that the exceptional point could be reached by the manipulation of such parameter by means of the twist, as occur in our original model.

The low-energy Hamiltonian then acquires the form

$$\mathcal{H}_{\mathbf{k}} = \begin{pmatrix} h_{\mathbf{k}}^{(+)} & T_1 & T_2 & T_3 \\ T_1 & h_{\mathbf{k}_1}^{(-)} & 0 & 0 \\ T_2 & 0 & h_{\mathbf{k}_2}^{(-)} & 0 \\ T_3 & 0 & 0 & h_{\mathbf{k}_3}^{(-)} \end{pmatrix},$$

with the tunneling term given by the off-diagonal terms in the Hamiltonian (3) in the main text. Following the Bistritzer-MacDonald (BM) [4] approach in the same way as in the main text (see also Sec. S3 of the SI), we find the effective low-energy Hamiltonian

$$\mathcal{H}_{\mathbf{k}}^{\text{eff}} = (v_{\text{H}}^* + v_{\text{NH}}^*\sigma_3)\boldsymbol{\sigma} \cdot \mathbf{k} + i\gamma^*, \quad (\text{S17})$$

where we identify the renormalized parameters:

$$\begin{aligned} \frac{v_{\text{H}}^*}{v} &= \frac{(1 + \bar{\gamma}^2)^2 - 3(\alpha_1^2 + \alpha_0^2\bar{\gamma}^2)}{(1 + \bar{\gamma}^2)^2 + 3(\alpha_0^2 + \alpha_1^2)(1 - \bar{\gamma}^2)}, \\ \frac{v_{\text{NH}}^*}{v} &= -\frac{6\alpha_0\alpha_1\bar{\gamma}}{(1 + \bar{\gamma}^2)^2 + 3(\alpha_0^2 + \alpha_1^2)(1 - \bar{\gamma}^2)}, \\ \frac{\gamma^*}{\gamma} &= 1 - 3\frac{(\alpha_0^2 + \alpha_1^2)}{(1 + \bar{\gamma}^2)}. \end{aligned}$$

Here,  $\alpha_i = w_i/vk_{\theta}$  and similarly  $\bar{\gamma} = \gamma/vk_{\theta}$ . As can be seen, the gain-loss contribution leads to an emergent non-Hermitian term that is equivalent to the non-reciprocal hopping model in Eq. (11) of the main text, up to the on-site dissipative term  $\sim \gamma^*$ . Moreover, the dissipation parameter  $\gamma$  in Eq. (S16) can always be conveniently chosen so that  $\gamma^* = 0$  for any angle, with which the system

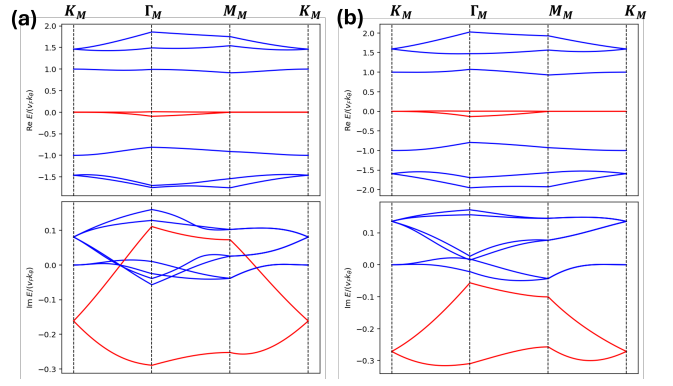

Figure S5. Band structure at the HMA for  $w_0 \neq 0$ , specifically (a)  $\alpha_0 = 0.2$  and (b)  $\alpha_0 = 0.4$ . Notice that in both cases the bands remain flat with little to no modification of the real part of the spectrum. The main difference between them comes from the imaginary part, that exhibits a displacement of the corresponding flat bands (red and purple curves in both plots) proportional to the value of  $\alpha_0$ .

becomes equivalent to our minimal model (Eq. (11) in the main text). As such, the two models belong to the same class of non-Hermitian realizations of TBG.

A second possibility is to consider sublattice dissipation, with the Hamiltonian for both layers given by

$$h_{\mathbf{k}} = v\boldsymbol{\sigma} \cdot \mathbf{k} + i\gamma\sigma_3, \quad (\text{S18})$$

while the on-site dissipation is asymmetric between the two sublattices. In this case, the spectrum is given by  $\epsilon_{\mathbf{k}} = \sqrt{v^2|\mathbf{k}|^2 - \gamma^2}$ , and thus the dissipative term  $\gamma$  acts as an effective “imaginary mass”. A specific feature of this model is that the exceptional points are momentum dependent, lying on the circle  $|\mathbf{k}| = \gamma/v \equiv k_e$ . The spectrum is also purely real or imaginary for  $|\mathbf{k}| > k_e$  and  $|\mathbf{k}| < k_e$ , respectively. Thus, we may expect that the phenomenology in this case to be different from the previous scenarios.

By following the BM approach in the same manner of our previous calculations, we find the effective Hamiltonian

$$\mathcal{H}_{\mathbf{k}}^{\text{eff}} = v^*\boldsymbol{\sigma} \cdot \mathbf{k} + i\gamma^*\sigma_3, \quad (\text{S19})$$

with renormalized parameters

$$\begin{aligned} \frac{v^*}{v} &= \frac{(1 - \bar{\gamma}^2)^2 - 3(\alpha_1^2 - \alpha_0^2\bar{\gamma}^2)}{(1 - \bar{\gamma}^2)(1 - \bar{\gamma}^2 + 3\alpha_0^2 + 3\alpha_1^2)}, \\ \frac{\gamma^*}{\gamma} &= 1 + 3\frac{(\alpha_0^2 - \alpha_1^2)}{(1 - \bar{\gamma}^2)}. \end{aligned}$$

In this case there is no emergence of non-Hermitian velocity, and thus there is no direct equivalence with the previous models. The models in Eq. (S16) and Eq. (S19) therefore belong to different classes of non-Hermitian versions of TBG. As can be seen, the spectrum for this model

can also be driven to its exceptional points by tuning the two independent parameters  $\gamma$  and  $\theta$ , and therefore it also features the exceptional magic angles. Specifically, by turning off the dissipative term in Eq. (S19), and therefore choosing  $1 - \tilde{\gamma}^2 = 3(\alpha_1^2 - \alpha_0^2)$ , the form of  $v^*$  reduces to

$$\frac{v^*}{v} = \frac{3\alpha_1^2 - 6\alpha_0^2 - 1}{6\alpha_1^2},$$

where the magic angle in the chiral limit  $\alpha_0 = 0$  is again given by the known result  $\alpha_1 = 1/\sqrt{3}$ .

In summary, although there are at least two different classes of non-Hermitian versions of TBG, all of them exhibit the emergence of EMAs. However, our original non-reciprocal hopping model is minimal in the sense that it requires fine-tuning of only one parameter, the twist angle, to reach the EMAs.

## S7. EXPERIMENTAL PROPOSAL

Motivated by the recent experimental observation of moiré physics induced by relative twist of optical lattices [6], we propose to include non-Hermiticity by adding two auxiliary optical lattices, each of them coupled to a monolayer of the main system and connected to external reservoirs, inducing dissipation in the original (without auxiliary lattices) bilayer system. Specifically, taking into account the auxiliary lattice, the tight-binding model for the monolayer NH graphene lattice becomes

$$H^{(s)} = \sum_{\langle i,j \rangle} t_{ab}(a_i^\dagger b_j + h.c.) + \sum_i (t_{ac}e^{i\phi}c_i^\dagger a_i + t_{bc}c_i^\dagger b_i + h.c. + (\Delta + is\gamma)c_i^\dagger c_i), \quad (\text{S20})$$

where the first term is the standard nearest-neighbors hopping Hamiltonian, and the second term describes the interaction between the monolayer and its auxiliary lattice, such as  $is\gamma$  stands for the gain ( $s = +$ ) or loss ( $s = -$ ) induced by the coupling to external reservoirs. Parameters  $\Delta$ ,  $t_{ab}$ ,  $t_{bc}$  and  $t_{ac}$  can be separately tuned through Raman or Bragg processes, and the phase  $e^{i\phi}$  arises from the effective magnetic flux through the closed loop formed by sites  $a$ ,  $b$  and  $c$ , as explicitly shown in Appendix of Ref. [7]. Notice that integration over the auxiliary degrees of freedom  $c_i$  or, equivalently, projection over the Hilbert subspace of the original lattice through the

Schur complement leads to the effective Hamiltonian [7]

$$H_{\text{eff}}^{(s)} = \sum_i \Delta_a a_i^\dagger a_i + \sum_j \Delta_b b_j^\dagger b_j + \sum_{\langle i,j \rangle} (\tilde{t}_{ab} a_i^\dagger b_j + \tilde{t}_{ba} b_j^\dagger a_i), \quad (\text{S21})$$

with complex on-site energies  $\Delta_\alpha = t_{\alpha c}^2 \tilde{\Delta}$ , where  $\tilde{\Delta} = (\Delta - is\gamma)/(\Delta^2 + \gamma^2)$  for  $\alpha = a, b$ , and effective non-reciprocal complex hoppings  $\tilde{t}_{ab} = t_{ab} - t_{ac}t_{bc}e^{i\phi}\tilde{\Delta}$  and  $\tilde{t}_{ba} = t_{ab} - t_{ac}t_{bc}e^{-i\phi}\tilde{\Delta}$ . The two layers described by this model are then coupled with a Hermitian interlayer term (Eq. (3) in the main text), which was realized in the experiment in Ref. [6].

As our analysis explicitly shows, the emergence of exceptional magic angles is expected by fine tuning the physical parameters in the experimental setup. In particular, this can be achieved by choosing  $\Delta = 0$ , the difference of hopping amplitudes  $\delta t = (t_{ab} - \tilde{t}_{ba})/2 = -st_{ac}t_{bc}\sin(\phi)/\gamma \in \mathbb{R}$ , and the dissipation at each site in the layer  $s = \pm$  proportional to  $-is/\gamma$ . Therefore, the Hamiltonian describing the proposed experimental setup reduces to an effective non-reciprocal hopping model with on-site gain/loss, Eq. (S16).

- 
- [1] D. C. Brody, Biorthogonal quantum mechanics, *Journal of Physics A: Mathematical and Theoretical* **47**, 035305 (2013).
  - [2] V. M. Martinez Alvarez, J. E. Barrios Vargas, and L. E. F. Foa Torres, Non-hermitian robust edge states in one dimension: Anomalous localization and eigenspace condensation at exceptional points, *Phys. Rev. B* **97**, 121401 (2018).
  - [3] E. J. Bergholtz, J. C. Budich, and F. K. Kunst, Exceptional topology of non-hermitian systems, *Rev. Mod. Phys.* **93**, 015005 (2021).
  - [4] R. Bistritzer and A. H. MacDonald, Moiré bands in twisted double-layer graphene, *Proceedings of the National Academy of Sciences* **108**, 12233 (2011).
  - [5] K. Kawabata, K. Shiozaki, M. Ueda, and M. Sato, Symmetry and Topology in Non-Hermitian Physics, *Phys. Rev. X* **9**, 041015 (2019).
  - [6] Z. Meng, L. Wang, W. Han, F. Liu, K. Wen, C. Gao, P. Wang, C. Chin, and J. Zhang, Atomic Bose-Einstein condensate in twisted-bilayer optical lattices, *Nature* **615**, 231 (2023).
  - [7] Q. Liang, D. Xie, Z. Dong, H. Li, H. Li, B. Gadway, W. Yi, and B. Yan, Dynamic Signatures of Non-Hermitian Skin Effect and Topology in Ultracold Atoms, *Phys. Rev. Lett.* **129**, 070401 (2022).
